# Supplementary material for: Self-Paced Learning: an Implicit Regularization Perspective
Source: arXiv:1606.00128 source file (2016-09-18)
Supplement: Supplementary file 1 [file appendix.tex]

\clearpage
\section*{Supplementary Materials}

%\title{Self-Paced Learning via Implicit Optimization}
%\title{Supplementary Materials for \\ Self-Paced Learning: an Implicit Regularization Perspective}

Similar definitions of self-paced regularizer (or self-paced function) have been proposed in \cite{jiang2014easy,jiang2015self,zhao2015self}. The definition in \cite{zhao2015self} is given below.

\textbf{Definition (Self-Paced Regularizer)} \cite{zhao2015self}: Suppose that $v$ is a weight variable, $\ell$ is the loss, and $\lambda$ is the learning pace parameter. $g(v,\lambda)$ is called self-paced rgularizer, if
\begin{spacing}{1.0} 
	\emph{1. \(g(v, \lambda)\) is convex with respect to $v \in [0,1]$;} 
	
	\emph{2. $v^*(\lambda, \ell)$ is monotonically decreasing with respect to $\ell$, and it holds that $\lim_{\ell \to 0} v^*(\lambda, \ell)$} = 1,
	\emph{$\lim_{\ell \to \infty} v^*(\lambda, \ell)$} = 0 \emph{;} 
	
	\emph{3. $v^*(\lambda, \ell)$ is monotonically increasing with respect to ${\lambda}$, and it holds that $\lim_{\lambda \to 0} v^*(\lambda, \ell)$} = 0, \emph{$\lim_{\lambda \to \infty} v^*(\lambda, \ell) \leq $} 1 \emph{;} 
		
	\emph{where $v^*(\lambda, \ell) = \arg\min_{v \in [0,1]} v\ell + g(v,\lambda)$.}
\end{spacing}

Table \ref{existed_spl_regularizer} tabulates some recently proposed self-paced regularizers $g(v, \lambda)$ and their corresponding $v^*(\lambda, \ell)$.
We modify their original expressions for better comparison.

Figure \ref{fig:mf_result} shows the curves of some loss functions and their corresponding minimizer functions.

\begin{figure*}[tbh]
	\setlength{\abovecaptionskip}{0pt}
	\setlength{\belowcaptionskip}{-5pt}
	\centering
	\subfigure{
		\includegraphics[height=1.8in]{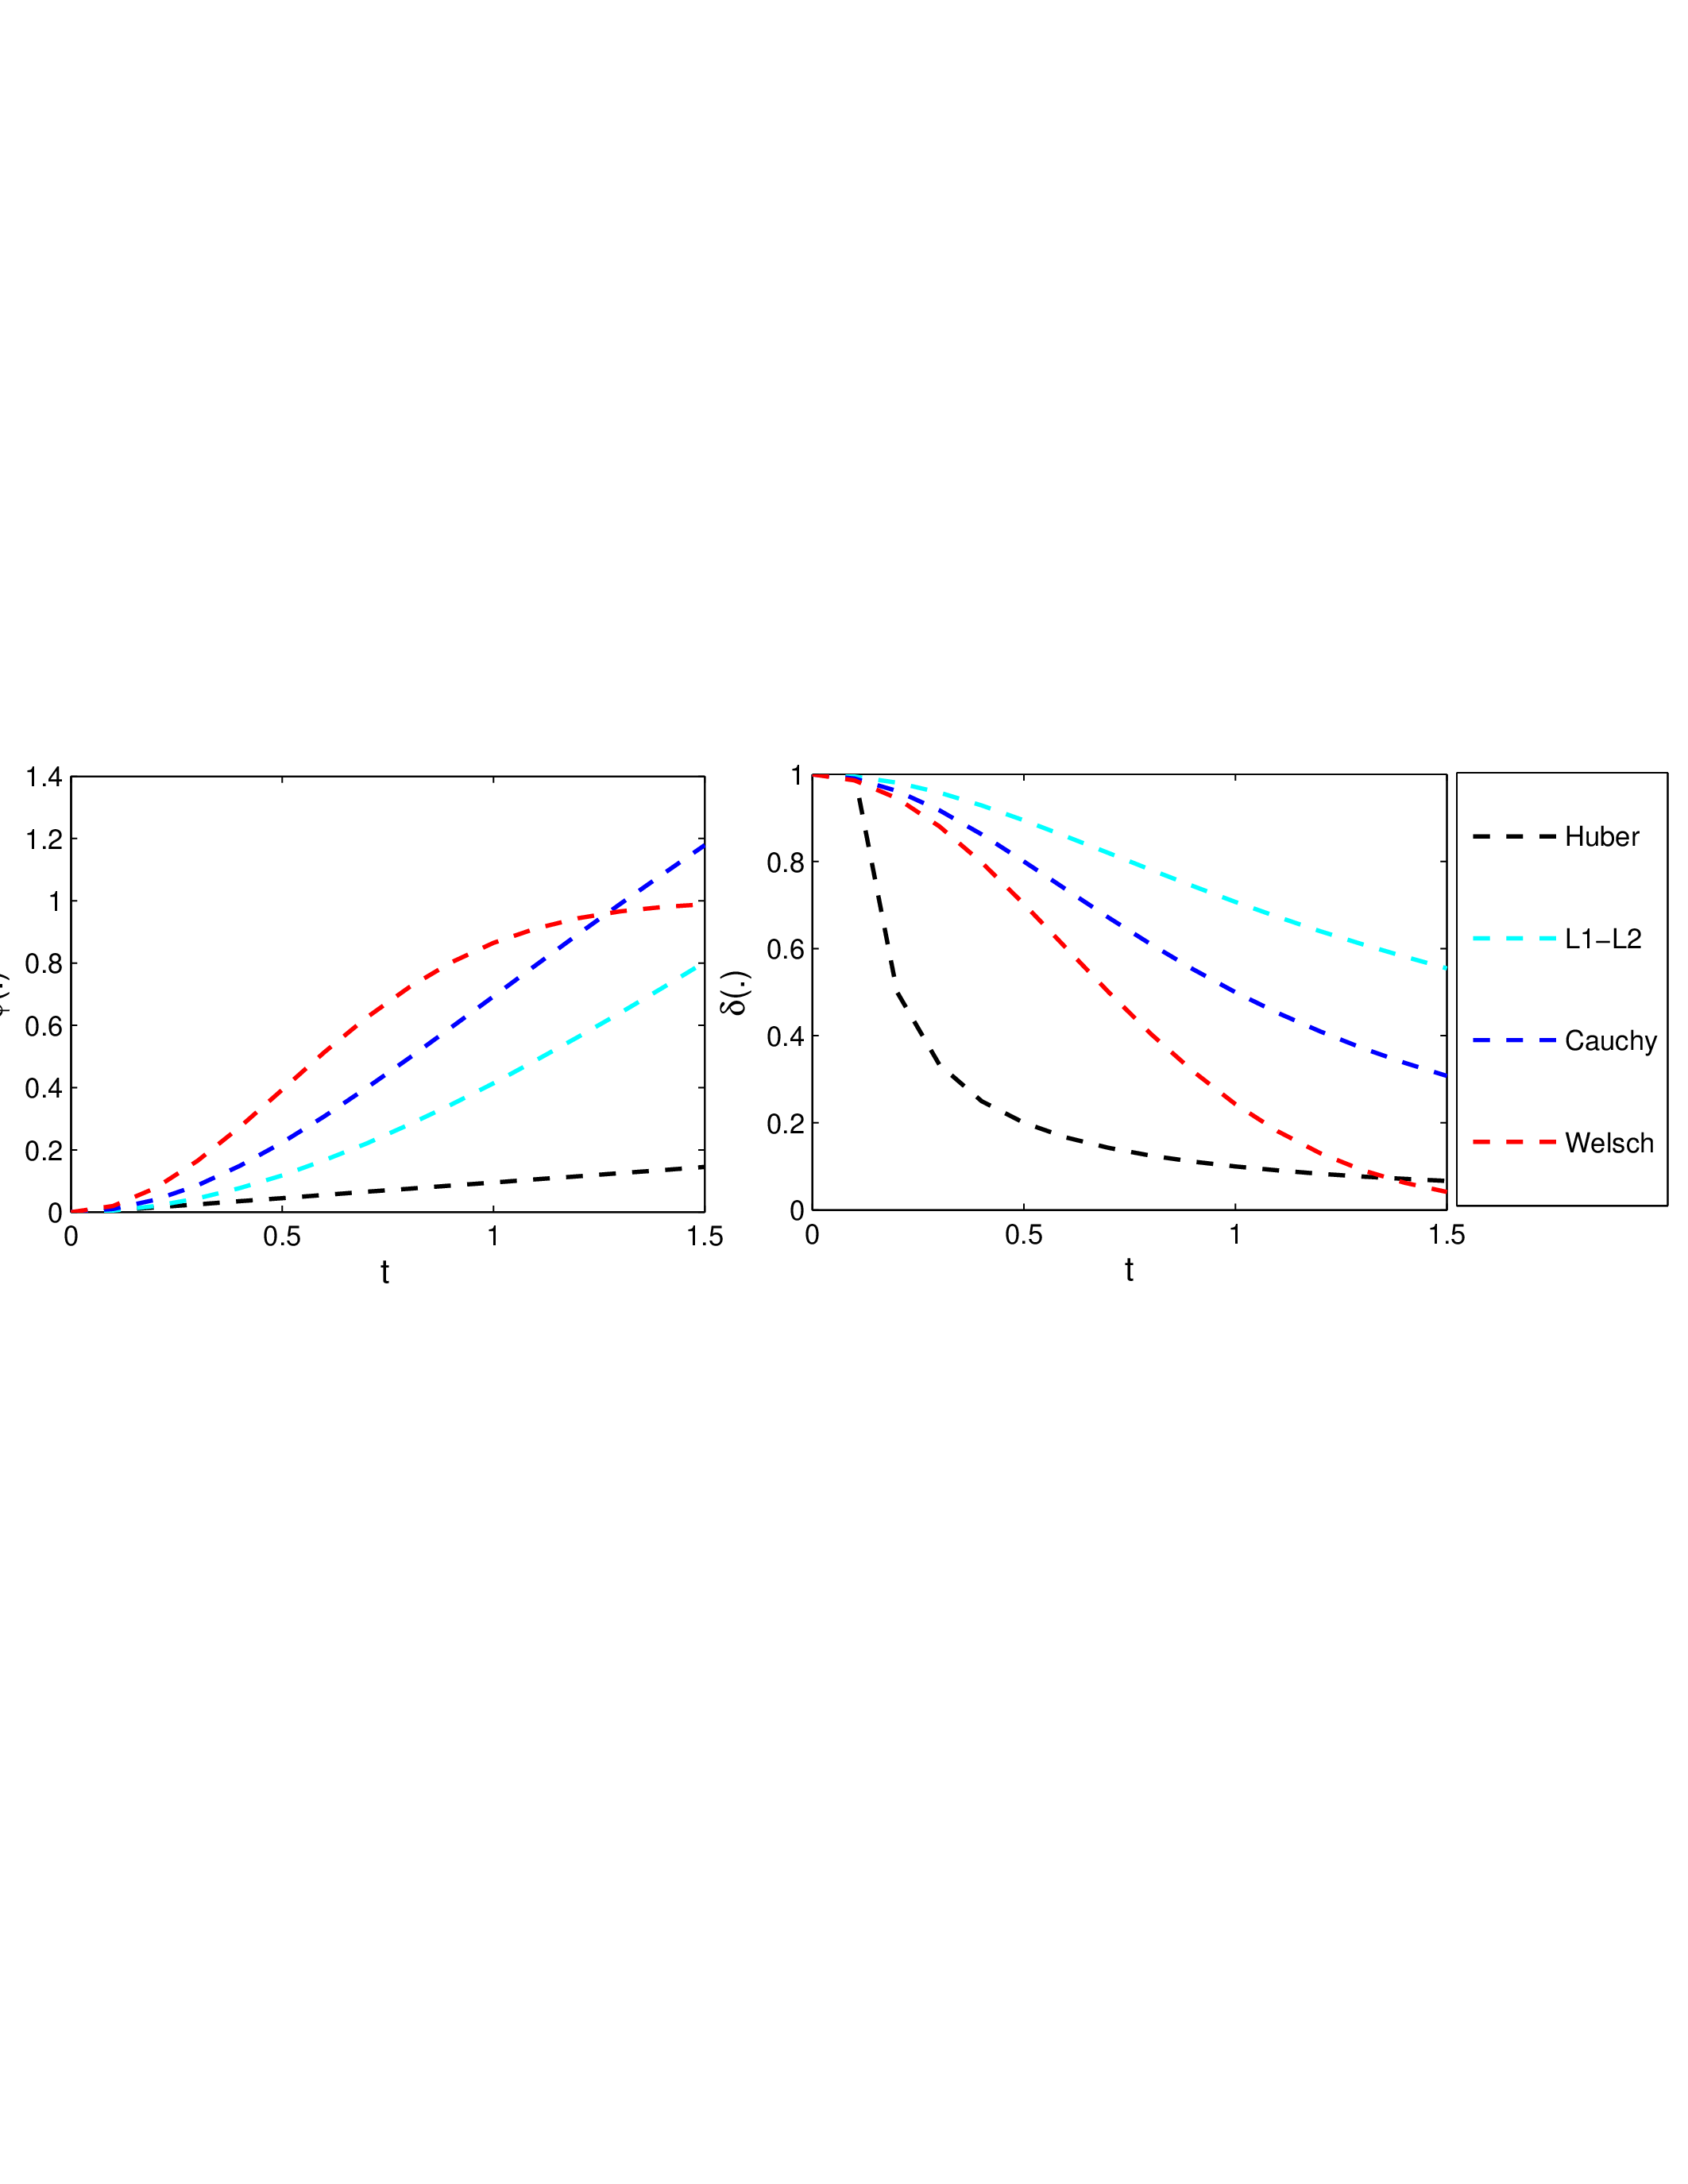}
	}
	
	\caption{Loss Function $\phi(.)$ and the Corresponding Minimizer Function $\delta(.)$.}
	\label{fig:mf_result}
\end{figure*}

\begin{table}
\footnotesize
\centering
\caption{Recently Proposed Self-paced Regularizers and their Corresponding Minimizer Functions}
\label{existed_spl_regularizer}
\setlength\tabcolsep{2pt}
\begin{tabular}{|l|l|l|}

%
%regularization and minimization function
\hline
	& Self-paced Regularizer $g(.)$	& Minimizer Function $\sigma(.)$ \\

%hard
\hline
Kumar \etal \cite{kumar2010self}
& 	

$-\lambda \sum_{i=1}^{n} v_i,\ \lambda>0$

&
$\left\{ {\begin{array}{*{20}{c}}
	1, &  \ell_i < \lambda \\
	0, &  otherwise
	\end{array}} 
\right.$
\\

%linear
\hline
Lu Jiang \etal \cite{jiang2014easy,jiang2015self}

&
$\frac{1}{2} \lambda \sum_{i=1}^{n} (v_i^2 - 2v_i), \ \lambda > 0 $

&
$\left\{ {\begin{array}{*{20}{c}}
	1 - \frac{1}{\lambda}\ell_i, &  \ell_i < \lambda \\
	0, &  otherwise
	\end{array}} 
\right.$
\\

%logarithmic
\hline
Lu Jiang \etal \cite{jiang2014easy,jiang2015self}

&
$\begin{aligned}
&\sum_{i=1}^{n}( \zeta v_i - \frac{\zeta^{v_i}}{\log \zeta}), \\
&\zeta = 1 - \lambda, 0 < \lambda < 1 
\end{aligned}$

&
$\left\{ {\begin{array}{*{20}{c}}
	\frac{1}{\log \zeta} \log(\ell_i + \zeta), &  \ell_i < \lambda \\
	0, &  otherwise
	\end{array}} 
\right.$
\\

%mixture
\hline
{Lu Jiang \etal \cite{jiang2014easy,jiang2015self} }

&

$\begin{aligned}
&-\zeta \sum_{i=1}^{n}\log(v_i + \frac{1}{\lambda_1}\zeta), \\
&\zeta = \frac{\lambda_1 \lambda_2}{\lambda_1 - \lambda_2}, \lambda_1 > \lambda_2 >0
\end{aligned}
$

&
$\left\{ {\begin{array}{*{20}{c}}
	1, &  \ell_i \leq \lambda_2 \\
	\frac{(\lambda_1 - \ell_i)\zeta}{\ell_i \lambda_1}, & \lambda_2 < \ell_i < \lambda_1 \\
	0, &  \ell_i \geq \lambda_1
	\end{array}} 
\right.$
\\

%diversity
\hline
Lu Jiang \etal \cite{jiang2014self}

&
$-\lambda\sum_{i=1}^{n} v_i - \gamma||\bv||_{2,1}, \ \lambda > 0, \ \gamma > 0$

&
$\left\{ {\begin{array}{*{20}{c}}
	1, &  \ell_i \leq \lambda + \gamma \frac{1}{\sqrt{i} - \sqrt{i-1}} \\
	0, &  otherwise
	\end{array}} 
\right.$
\\

%multi-view clustering
\hline
Chang Xu \etal \cite{xu2015multi}

&
$\begin{aligned}
&\sum_{i=1}^{n} \ln(1 + e^{-\lambda} - v_i)^{(1 + e^{-\lambda} - v_i)} \\
&+ \ln(v_i)^{v_i} - \lambda v_i, \ \lambda > 0
\end{aligned}$

&
$\frac{1 + e^{-\lambda}}{1 + e^{\ell_i - \lambda}}$
\\

%matric factorization
\hline
Qian Zhao \etal \cite{zhao2015self}

&
$\sum_{i=1}^{n} \frac{\lambda \gamma^2}{\lambda v_i + \gamma}, \ \lambda > 0, \ \gamma > 0$

&
$\left\{ {\begin{array}{*{20}{c}}
	1, &  \ell_i \leq (\frac{\lambda \gamma}{\lambda + \gamma})^2 \\
	0, &  \ell_i \geq \lambda^2 \\
	\gamma (\frac{1}{\sqrt{\ell_i}} - \frac{1}{\lambda}), & otherwise 
	\end{array}} 
\right.$
\\

%co-saliency detection
\hline
Zhang \etal \cite{zhang2015self}

&
$\begin{aligned}
&-\lambda \sum_{k=1}^{K} \sum_{i=1}^{n_k} v_i^k -\gamma \sum_{k=1}^{K} \sqrt{\sum_{i=1}^{n_k} v_i^k},\\
&\lambda > 0, \ \gamma > 0
\end{aligned}$

&
$\left\{ {\begin{array}{*{20}{c}}
	1, &  \ell_i^k < \lambda + \frac{\gamma}{2\sqrt{i}} \\
	\frac{((\frac{\gamma}{2(\ell_i^k-\lambda)})^2 - (i-1)}{m}, &  otherwise
	\end{array}} 
\right.$
\\
\hline
\end{tabular}
\end{table}

%\section{Self-Paced Implicit Regularizer}
