# Supplementary material for: Self-Paced Learning: an Implicit Regularization Perspective
Source: arXiv:1606.00128 source file (2016-09-18)
Supplement: Supplementary file 3 [file databases.tex]

\begin{table} [tb]
	\footnotesize
	\caption{\small{Statistical Information of Databases.}}
	\centering
	\label{statistical_information_database}
	\begin{tabular}{|c|c|c|c|}
		\hline
		\textbf{Dataset} & \textbf{\#.Category} & \textbf{\#.Instance} & \textbf{\#.Feature} \\
		
		\hline
		Breast Wisconsion & 2 & 569 & 30 \\
		
		\hline
		Pima & 2 & 768 & 8 \\
		
		\hline
		Splice & 2 & 3175 & 60 \\
				
		\hline
		Spambase & 2 & 4601 & 57 \\
		
		\hline
		Phoneme & 2 & 5404 & 5 \\
		
		\hline
		Svmguide1 & 2 & 7089 & 4 \\
				
		\hline
	\end{tabular}
\end{table}
