# Supplementary material for: Self-Paced Learning: an Implicit Regularization Perspective
Source: arXiv:1606.00128 source file (2016-09-18)
Supplement: Supplementary file 7 [file math_alphabet.tex]

%math type 字体

\def\b0{\mathbf{0}}
\def\b1{\mathbf{1}}
