# Supplementary material for: Self-Paced Learning: an Implicit Regularization Perspective
Source: arXiv:1606.00128 source file (2016-09-18)
Supplement: Supplementary file 8 [file mystyle.tex]

\usepackage{epsfig}
\usepackage{graphicx}
\usepackage{amsmath}
\usepackage{amssymb}
\usepackage{amsthm}
\usepackage{graphicx}
\usepackage{slashbox}
\usepackage{subfigure}
\usepackage{rotating}

\usepackage{amssymb}
\usepackage{bm}

\usepackage{epstopdf}
\usepackage{stmaryrd}
\usepackage{amsfonts}
\usepackage{array}
\usepackage{amssymb}
\usepackage{algorithmic}
\usepackage{algorithm}
\usepackage{multirow}
\usepackage{color}
\usepackage{threeparttable}
\usepackage{enumerate}
\usepackage{mathrsfs}

\usepackage{tabularx}
\usepackage{makecell, rotating}

\usepackage{setspace}
\usepackage{chngpage}
\usepackage{graphics}
\usepackage{graphicx}
\usepackage{epsfig}

%algorithm
\usepackage[english]{babel}
\usepackage{blindtext}
\usepackage{algorithm} %format of the algorithm
\usepackage{algorithmic} %format of the algorithm

\def\b0{\mathbf{0}}
\def\b1{\mathbf{1}}

\makeatletter
\DeclareRobustCommand\onedot{\futurelet\@let@token\@onedot}
\def\@onedot{\ifx\@let@token.\else.\null\fi\xspace}
