# Supplementary material for: Self-Paced Learning: an Implicit Regularization Perspective
Source: arXiv:1606.00128 source file (2016-09-18)
Supplement: Supplementary file 11 [file table_classification.tex]

\begin{table*}[!htbh]
	\footnotesize
	\centering
	\caption{Classification Accuracy (\%).}
	\label{result_classification}
	\setlength\tabcolsep{2pt}
	
%	\begin{tabular}{c c c c c c c c c}
	\begin{tabular}{|c| c| c| c| c| c| c| c| c|}
		\hline
		\hline
		\multicolumn{9}{|c|}{Without Label Noise} \\
		
		\hline
		Method & \tabincell{c} {LR } & \tabincell{c}{SPL-hard}  & 
		\tabincell{c}{SPL-linear}  & \tabincell{c}{SPL-mixture} & 
		\tabincell{c}{SPL-IR-huber} & \tabincell{c}{SPL-IR-l1-l2} &
		\tabincell{c}{SPL-IR-cauchy} & \tabincell{c}{SPL-IR-welsch} \\
		\hline
		
		%00
		Breast  & 97.36 $\pm$ 2.22 	& 98.59 $\pm$ 1.11 	& 98.42 $\pm$ 1.54 	& 98.25 $\pm$ 1.65 	& \textbf{98.77 $\pm$ 1.19} 	& 97.90 $\pm$ 1.79 	& 98.42 $\pm$ 1.54 	& 98.25 $\pm$ 1.65 	\\ 
		Spambase  & 92.35 $\pm$ 1.47 	& 92.63 $\pm$ 1.08 	& 93.00 $\pm$ 1.24 	& 92.83 $\pm$ 1.44 	& 93.05 $\pm$ 1.25 	& 93.00 $\pm$ 1.36 	& 93.09 $\pm$ 1.41 	& \textbf{93.13 $\pm$ 1.34} 	\\ 
		Phoneme  & 74.98 $\pm$ 2.24 	& 76.74 $\pm$ 2.01 	& 75.87 $\pm$ 2.12 	& 77.74 $\pm$ 2.44 	& 76.20 $\pm$ 2.24 	& 75.61 $\pm$ 2.29 	& \textbf{77.94 $\pm$ 2.08} 	& 77.67 $\pm$ 2.10 	\\ 
		Svmguide1 & 95.39 $\pm$ 0.95 	& 95.39 $\pm$ 0.95 	& 95.43 $\pm$ 1.05 	& 95.51 $\pm$ 1.04 	& 95.57 $\pm$ 0.95 	& 95.57 $\pm$ 1.10 	& 95.65 $\pm$ 1.01 	& \textbf{95.68 $\pm$ 0.90} 	\\ 
		\hline
		
%		
%		\hline
%		\hline
%		\multicolumn{9}{|c|}{With 10\% Random Label Noise} \\
%		
%		
%		\hline
%		Method & \tabincell{c} {LR } & \tabincell{c}{SPL-hard}  & 
%		\tabincell{c}{SPL-linear}  & \tabincell{c}{SPL-mixture} & 
%		\tabincell{c}{SPL-IR-huber} & \tabincell{c}{SPL-IR-l1-l2} &
%		\tabincell{c}{SPL-IR-cauchy} & \tabincell{c}{SPL-IR-welsch} \\
%		\hline
%		%10
%		Breast  & 93.14 $\pm$ 2.94 	& 97.01 $\pm$ 2.49 	& 97.19 $\pm$ 2.21 	& 96.83 $\pm$ 2.45 	& 97.02 $\pm$ 2.33 	& 95.25 $\pm$ 2.23 	& 97.19 $\pm$ 2.21 	& \textbf{97.36 $\pm$ 2.05} 	\\ 
%		Spambase  & 90.50 $\pm$ 1.77 	& 92.72 $\pm$ 1.63 	& 92.31 $\pm$ 1.46 	& 91.87 $\pm$ 1.52 	& 91.81 $\pm$ 1.80 	& 91.55 $\pm$ 1.79 	& 91.83 $\pm$ 1.54 	& 92.20 $\pm$ 1.33 	\\ 
%		Phoneme  & 75.39 $\pm$ 2.54 	& 75.39 $\pm$ 2.54 	& 76.96 $\pm$ 2.31 	& 74.95 $\pm$ 2.24 	& 76.20 $\pm$ 2.48 	& 75.57 $\pm$ 2.54 	& 77.79 $\pm$ 2.11 	& 77.76 $\pm$ 1.75 	\\ 
%		Svmguide1 & 93.10 $\pm$ 0.91 	& 95.84 $\pm$ 0.98 	& 95.26 $\pm$ 1.21 	& 94.75 $\pm$ 1.09 	& 94.46 $\pm$ 0.92 	& 94.27 $\pm$ 0.97 	& 94.85 $\pm$ 1.07 	& 95.20 $\pm$ 1.00 	\\ 
%		\hline

		\hline
		\hline
		\multicolumn{9}{|c|}{With 20\% Random Label Noise} \\
		
		\hline
		Method & \tabincell{c} {LR } & \tabincell{c}{SPL-hard}  & 
		\tabincell{c}{SPL-linear}  & \tabincell{c}{SPL-mixture} & 
		\tabincell{c}{SPL-IR-huber} & \tabincell{c}{SPL-IR-l1-l2} &
		\tabincell{c}{SPL-IR-cauchy} & \tabincell{c}{SPL-IR-welsch} \\
		\hline
		%20
		Breast  & 92.08 $\pm$ 2.96 	& 96.83 $\pm$ 2.62 	& 97.36 $\pm$ 2.54 	& 96.66 $\pm$ 2.26 	& 95.25 $\pm$ 2.36 	& 94.19 $\pm$ 2.66 	& 97.54 $\pm$ 1.90 	& \textbf{97.89 $\pm$ 2.00} 	\\ 
		Spambase  & 89.28 $\pm$ 1.66 	& 91.52 $\pm$ 1.64 	& 91.22 $\pm$ 1.35 	& 90.44 $\pm$ 1.70 	& 90.31 $\pm$ 1.48 	& 90.02 $\pm$ 1.60 	& 90.65 $\pm$ 1.55 	& 91.20 $\pm$ 1.34 	\\ 
		Phoneme  & 74.93 $\pm$ 2.32 	& 76.18 $\pm$ 2.33 	& 76.35 $\pm$ 2.17 	& 76.37 $\pm$ 2.28 	& 75.22 $\pm$ 2.43 	& 75.06 $\pm$ 2.32 	& 75.20 $\pm$ 2.33 	& 76.28 $\pm$ 2.03 	\\ 
		Svmguide1 & 91.52 $\pm$ 0.65 	& 94.47 $\pm$ 1.01 	& 94.50 $\pm$ 1.05 	& 93.68 $\pm$ 0.89 	& 93.10 $\pm$ 0.79 	& 92.79 $\pm$ 0.73 	& 93.86 $\pm$ 1.04 	& 94.26 $\pm$ 0.84 	\\ 
		
		\hline
		
	\end{tabular}
	%	\captionsetup{justification=centering}
\end{table*}
