# Supplementary material for: Self-Paced Learning: an Implicit Regularization Perspective
Source: arXiv:1606.00128 source file (2016-09-18)
Supplement: Supplementary file 12 [file table_classification_00.tex]

\begin{table}[!htbh]
	\footnotesize
	\centering
	\caption{
		\small{Classification Accuracy (\%) without Noise.}
	}
	\label{result_classification_00}
	\setlength\tabcolsep{1.5pt}
	\begin{tabular}{|l|c|c|c|c|}

		\hline
		Method & \tabincell{c}{Breast \\ Wisconsion} & Spambase & Phoneme & Svmguide1 \\
		
		\hline
		
		\tabincell{l}{LR \\ }			&  97.36 $\pm$ 2.22   &		92.35 $\pm$ 1.47   &		74.98 $\pm$ 2.24   &		95.39 $\pm$ 0.95   \\
		
		\hline
		\tabincell{l}{SPL-\\hard}    	& 97.37 $\pm$ 2.36 	& 92.35 $\pm$ 1.47 	& 76.74 $\pm$ 2.01 	& 95.39 $\pm$ 0.95 	\\ 
				
		\hline
		\tabincell{l}{SPL-\\linear}    	& 98.07 $\pm$ 1.73 	& 92.70 $\pm$ 1.53 	& 75.87 $\pm$ 2.12 	& 95.43 $\pm$ 1.05 	\\ 
				
		\hline
		\tabincell{l}{SPL-\\mixture}    & 97.72 $\pm$ 2.01 	& 92.76 $\pm$ 1.52 	& 77.74 $\pm$ 2.44 	& 95.50 $\pm$ 1.05 	\\ 
				
		\hline
		\tabincell{l}{SPL-IR-\\huber}   & 98.25 $\pm$ 1.65 	& 92.83 $\pm$ 1.40 	& 76.20 $\pm$ 2.24 	& 95.42 $\pm$ 1.08 	\\ 
				
		\hline
		\tabincell{l}{SPL-IR-\\l1-l2}   & 97.72 $\pm$ 2.17 	& 92.87 $\pm$ 1.37 	& 75.61 $\pm$ 2.29 	& 95.51 $\pm$ 1.16 	\\

		\hline
		\tabincell{l}{SPL-IR-\\cauchy}  & 97.90 $\pm$ 1.79 	& 92.91 $\pm$ 1.45 	& 77.94 $\pm$ 2.08 	& 95.53 $\pm$ 1.00 	\\ 
				
		\hline
		\tabincell{l}{SPL-IR-\\welsch}  & 98.07 $\pm$ 1.53 	& 92.78 $\pm$ 1.41 	& 77.67 $\pm$ 2.10 	& 95.46 $\pm$ 0.99 	\\ 
										
		\hline
	\end{tabular}
\end{table}
