# Supplementary material for: Self-Paced Learning: an Implicit Regularization Perspective
Source: arXiv:1606.00128 source file (2016-09-18)
Supplement: Supplementary file 13 [file table_classification_10.tex]

\begin{table}[!htbh]
	\footnotesize
	\centering
	\caption{
		\small{Classification Accuracy (\%) with 10\% Label Noise.}
	}
	\label{result_classification_00}
	\setlength\tabcolsep{1.5pt}
	\begin{tabular}{|l|c|c|c|c|}

		\hline
		Method & \tabincell{c}{Breast \\ Wisconsion} & Spambase & Phoneme & Svmguide1 \\
		
		\hline
		
		\tabincell{l}{LR \\ }			&  93.14 $\pm$ 2.94   &		90.50 $\pm$ 1.77  	&		75.39 $\pm$ 2.54  	&		93.10 $\pm$ 0.91  	\\
		
		\hline
		\tabincell{l}{SPL-\\hard}    	& 96.13 $\pm$ 2.31 	& 92.72 $\pm$ 1.63 	& 75.39 $\pm$ 2.54 	& 95.84 $\pm$ 0.98 	\\ 
				
		\hline
		\tabincell{l}{SPL-\\linear}    	&  97.36 $\pm$ 2.22   &		92.35 $\pm$ 1.47   &		74.98 $\pm$ 2.24   &		95.39 $\pm$ 0.95   \\
				
		\hline
		\tabincell{l}{SPL-\\mixture}    &  97.36 $\pm$ 2.22   &		92.35 $\pm$ 1.47   &		74.98 $\pm$ 2.24   &		95.39 $\pm$ 0.95   \\
				
		\hline
		\tabincell{l}{SPL-IR-\\huber}   &  97.36 $\pm$ 2.22   &		92.35 $\pm$ 1.47   &		74.98 $\pm$ 2.24   &		95.39 $\pm$ 0.95   \\
				
		\hline
		\tabincell{l}{SPL-IR-\\l1-l2}   &  97.36 $\pm$ 2.22   &		92.35 $\pm$ 1.47   &		74.98 $\pm$ 2.24   &		95.39 $\pm$ 0.95   \\

		\hline
		\tabincell{l}{SPL-IR-\\cauchy}  &  97.36 $\pm$ 2.22   &		92.35 $\pm$ 1.47   &		74.98 $\pm$ 2.24   &		95.39 $\pm$ 0.95   \\
				
		\hline
		\tabincell{l}{SPL-IR-\\welsch}  &  97.36 $\pm$ 2.22   &		92.35 $\pm$ 1.47   &		74.98 $\pm$ 2.24   &		95.39 $\pm$ 0.95   \\
										
		\hline
	\end{tabular}
\end{table}
