# Supplementary material for: Self-Paced Learning: an Implicit Regularization Perspective
Source: arXiv:1606.00128 source file (2016-09-18)
Supplement: Supplementary file 15 [file table_classification_small.tex]

\begin{table*}[!htbh]
	\footnotesize
	\centering
	\caption{Classification Accuracy (\%).}
	\label{result_classification}
	\setlength\tabcolsep{5pt}
	
%	\begin{tabular}{c c c c c c c c c}
	\begin{tabular}{|c| c| c| c| c| c| c|}
		\hline
		\hline
		\multicolumn{7}{|c|}{Without Label Noise} \\
		
		\hline
		Method & \tabincell{c} {LR }  & \tabincell{c}{SPL-hard} & \tabincell{c}{SPL-mixture} & 
		\tabincell{c}{SPL-IR-huber} & \tabincell{c}{SPL-IR-l1-l2} &
		\tabincell{c}{SPL-IR-cauchy} & \tabincell{c}{SPL-IR-welsch} \\
		\hline
		
		%00
		Breast  & 97.36 $\pm$ 2.22 & 97.54 $\pm$ 2.22 &	& 98.25 $\pm$ 1.65 	& \textbf{98.77 $\pm$ 1.19} 	& 97.90 $\pm$ 1.79 	& 98.42 $\pm$ 1.54 	& 98.25 $\pm$ 1.65 	\\ 
		Spambase  & 92.35 $\pm$ 1.47 & 92.63 $\pm$ 1.08 &	& 92.83 $\pm$ 1.44 	& 93.05 $\pm$ 1.25 	& 93.00 $\pm$ 1.36 	& 93.09 $\pm$ 1.41 	& \textbf{93.13 $\pm$ 1.34} 	\\ 
%		Phoneme  & 74.98 $\pm$ 2.24 	& 77.74 $\pm$ 2.44 	& 76.20 $\pm$ 2.24 	& 75.61 $\pm$ 2.29 	& \textbf{77.94 $\pm$ 2.08} 	& 77.67 $\pm$ 2.10 	\\ 
		Svmguide1 & 95.39 $\pm$ 0.95 & 95.39 $\pm$ 0.95 &	& 95.51 $\pm$ 1.04 	& 95.57 $\pm$ 0.95 	& 95.57 $\pm$ 1.10 	& 95.65 $\pm$ 1.01 	& \textbf{95.68 $\pm$ 0.90} 	\\ 
		\hline
		
%		
%		\hline
%		\hline
%		\multicolumn{9}{|c|}{With 10\% Random Label Noise} \\
%		
%		
%		\hline
%		Method & \tabincell{c} {LR } & \tabincell{c}{SPL-hard}  & 
%		\tabincell{c}{SPL-linear}  & \tabincell{c}{SPL-mixture} & 
%		\tabincell{c}{SPL-IR-huber} & \tabincell{c}{SPL-IR-l1-l2} &
%		\tabincell{c}{SPL-IR-cauchy} & \tabincell{c}{SPL-IR-welsch} \\
%		\hline
%		%10
%		Breast  & 93.14 $\pm$ 2.94 	& 97.01 $\pm$ 2.49 	& 97.19 $\pm$ 2.21 	& 96.83 $\pm$ 2.45 	& 97.02 $\pm$ 2.33 	& 95.25 $\pm$ 2.23 	& 97.19 $\pm$ 2.21 	& \textbf{97.36 $\pm$ 2.05} 	\\ 
%		Spambase  & 90.50 $\pm$ 1.77 	& 92.72 $\pm$ 1.63 	& 92.31 $\pm$ 1.46 	& 91.87 $\pm$ 1.52 	& 91.81 $\pm$ 1.80 	& 91.55 $\pm$ 1.79 	& 91.83 $\pm$ 1.54 	& 92.20 $\pm$ 1.33 	\\ 
%		Phoneme  & 75.39 $\pm$ 2.54 	& 75.39 $\pm$ 2.54 	& 76.96 $\pm$ 2.31 	& 74.95 $\pm$ 2.24 	& 76.20 $\pm$ 2.48 	& 75.57 $\pm$ 2.54 	& 77.79 $\pm$ 2.11 	& 77.76 $\pm$ 1.75 	\\ 
%		Svmguide1 & 93.10 $\pm$ 0.91 	& 95.84 $\pm$ 0.98 	& 95.26 $\pm$ 1.21 	& 94.75 $\pm$ 1.09 	& 94.46 $\pm$ 0.92 	& 94.27 $\pm$ 0.97 	& 94.85 $\pm$ 1.07 	& 95.20 $\pm$ 1.00 	\\ 
%		\hline

		\hline
		\hline
		\multicolumn{7}{|c|}{With 20\% Random Label Noise} \\
		
		\hline
		Method & \tabincell{c} {LR } & \tabincell{c}{SPL-hard} & \tabincell{c}{SPL-mixture} & 
		\tabincell{c}{SPL-IR-huber} & \tabincell{c}{SPL-IR-L1-L2} &
		\tabincell{c}{SPL-IR-cauchy} & \tabincell{c}{SPL-IR-welsch} \\
		\hline
		%20
		Breast  & 92.08 $\pm$ 2.96 	& 96.13 $\pm$ 2.15 & 96.66 $\pm$ 2.26 	& 96.84 $\pm$ 2.33 	& 94.92 $\pm$ 2.89 	& 97.54 $\pm$ 1.90 	& \textbf{97.89 $\pm$ 1.63} 	\\ 
		Spambase  & 89.28 $\pm$ 1.66  & 89.81 $\pm$ 1.61 &	& 90.76 $\pm$ 1.82 	&  90.92 $\pm$ 1.65	& 90.09 $\pm$ 1.65 	& 90.85 $\pm$ 1.55 	& \textbf{91.37 $\pm$ 1.37} 	\\ 
%		Phoneme  & 74.61 $\pm$ 2.55 	& 77.31 $\pm$ 2.69 	& 75.26 $\pm$ 2.65 	& 75.07 $\pm$ 2.56 	& 75.91 $\pm$ 2.74 	& 77.89 $\pm$ 2.14 	\\ 
		Svmguide1 & 91.52 $\pm$ 0.65  & 92.72 $\pm$ 1.12 &	& 93.81 $\pm$ 0.79 	& 93.54 $\pm$ 0.75 	& 92.83 $\pm$ 0.71 	& 93.88 $\pm$ 1.05 	& \textbf{94.37 $\pm$ 0.90} 	\\ 
		
		\hline
		
	\end{tabular}
	%	\captionsetup{justification=centering}
\end{table*}
