# Supplementary material for: Self-Paced Learning: an Implicit Regularization Perspective
Source: arXiv:1606.00128 source file (2016-09-18)
Supplement: Supplementary file 16 [file table_classification_small_2.tex]

\begin{table}[!htbh]
	\footnotesize
	\centering
	\caption{Classification accuracy (\%). The best results are highlighted in bold, respectively.}
	\label{result_classification}
	\setlength\tabcolsep{4pt}
	
%	\begin{tabular}{c c c c c c c c c}
	\begin{tabular}{|l| c| c| c|}
		\hline
		\multicolumn{4}{|c|}{Without Label Noise} \\
		
		\hline
		Method & \tabincell{c}{Breast} & Spambase & Svmguide1 \\
		
		\hline
		
		\tabincell{l}{LR }			  & 97.36 $\pm$ 2.22 &		92.35 $\pm$ 1.47 &		95.39 $\pm$ 0.95  \\
				
		\hline
		\tabincell{l}{SPL-mixture}    & 98.25 $\pm$ 1.65 	& 92.83 $\pm$ 1.44 	& 95.51 $\pm$ 1.04 	\\ 
				
		\hline
		\tabincell{l}{SPL-IR-huber}   & \textbf{98.77 $\pm$ 1.19} 	& 93.05 $\pm$ 1.25 	& 95.57 $\pm$ 0.95 	\\ 
				
		\hline
		\tabincell{l}{SPL-IR-l1-l2}   & 97.90 $\pm$ 1.79 	& 93.00 $\pm$ 1.36 	& 95.57 $\pm$ 1.10 	\\

		\hline
		\tabincell{l}{SPL-IR-cauchy}  & 98.42 $\pm$ 1.54 	& 93.09 $\pm$ 1.41 	& 95.65 $\pm$ 1.01 	\\ 
				
		\hline
		\tabincell{l}{SPL-IR-welsch}  & 98.25 $\pm$ 1.65 	& \textbf{93.13 $\pm$ 1.34} 	& \textbf{95.68 $\pm$ 0.90} 	\\

		%20
		\hline
		\multicolumn{4}{|c|}{With 20\% Random Label Noise} \\
		
		\hline
		Method & \tabincell{c}{Breast} & Spambase & Svmguide1 \\
		
		\hline
		
		\tabincell{l}{LR }			  & 92.08 $\pm$ 2.96 &	89.28 $\pm$ 1.66 &		91.52 $\pm$ 0.65 \\
				
		\hline
		\tabincell{l}{SPL-mixture}    & 96.66 $\pm$ 2.12 	& 90.76 $\pm$ 1.82 	& 93.81 $\pm$ 0.79 	\\ 
				
		\hline
		\tabincell{l}{SPL-IR-huber}   & 96.84 $\pm$ 2.33 	& 90.92 $\pm$ 1.65 	& 93.54 $\pm$ 0.75 	\\ 
				
		\hline
		\tabincell{l}{SPL-IR-l1-l2}   & 94.19 $\pm$ 2.66 	& 90.09 $\pm$ 1.65 	& 92.83 $\pm$ 0.71 	\\

		\hline
		\tabincell{l}{SPL-IR-cauchy}  & 97.54 $\pm$ 1.90 	& 90.85 $\pm$ 1.55 	& 93.88 $\pm$ 1.05 	\\ 
				
		\hline
		\tabincell{l}{SPL-IR-welsch}  & \textbf{97.89 $\pm$ 1.63} 	& \textbf{91.37 $\pm$ 1.37} 	& \textbf{94.37 $\pm$ 0.90} 	\\ 
		
		\hline
		
	\end{tabular}
	%	\captionsetup{justification=centering}
\end{table}
